# Supplementary material for: Robust Active Distillation
Source: arXiv:2210.01213 source file (2023-02-04)
Supplement: Supplementary file 3 [file general_penalty.tex]

\subsection{Proof of Theorem~\ref{thm:minimax-max-gain}}

\minimaxmaxgain
\begin{proof}
The proof relies on the the Minimax Theorem~\cite{neumann1928theorie}, which yields
$$
\min_{c\in\Delta_{n-m}} \max_{p\in\Delta_1} f(p,c) = \max_{p\in\Delta_1} \min_{c\in\Delta_{n-m}} f(p,c).
$$
We will further use two claims, which we'll prove shortly.

\begin{Claim}\label{claim:p}
Let $p^*$, $k^*$, and $N(k)$ be defined as in the statement of the lemma. Then $p^*\in\Delta_1$ and $N(k^*) = \min_{c\in\Delta_{n-m}} f(p^*, c)$.
\end{Claim}

\begin{Claim}\label{claim:c}
Let $k^*$ and $N(k)$ be defined as in the statement of the lemma. Further, define
\begin{align*}
c^*_i =& \begin{cases}
    \frac{N(k^*)+\ell_i}{g_i + \ell_i} \mbox{\ \ if $i\leq k^*$}    \\
    1 \mbox{\ \ otherwise}
    \end{cases}
\end{align*}
Then $c^*\in\Delta_{n-m}$ and
$N(k^*) = \max_{p\in\Delta_1} f(p, c^*)$.
\end{Claim}
Given the claims, we see
\begin{align*}
N(k^*) = \min_{c\in\Delta_{n-m}} f(p^*, c) 
    \leq& \max_{p\in\Delta_1} \min_{c\in\Delta_{n-m}} f(p, c) \mbox{\ \ by Claim~\ref{claim:p}} \\
    =& \min_{c\in\Delta_{n-m}}\max_{p\in\Delta_1} f(p, c) \mbox{\ \ by Minimax} \\
    \leq& \max_{p\in\Delta_1} f(p, c^*) = N(k^*) \mbox{\ \ by Claim~\ref{claim:c}}
\end{align*}
That is, $p^*$ attains the maximum, which is $N(k^*)$, as we wanted.

We now prove the claims.
Before beginning, we will first simplify $f(p,c)$ somewhat, finding
\begin{align*}
f(p, c) 
    =& \sum_i g_i p_i c_i - \sum_i \ell_i p_i (1-c_i)\\
    =& \sum_i (c_i(g_i + \ell_i) - \ell_i) p_i
\end{align*}
\begin{proof}[Proof of Claim~\ref{claim:p}]
We first show $p^*\in\Delta_1$. We have
\begin{align*}
\sum_{i\leq n} p^*_i = \sum_{i\leq k^*} p^*_i 
    = \sum_{i\leq k^*} \frac{1}{H_{k^*}(g_i+\ell_i)} 
    = \frac{H_{k^*}}{H_{k^*}} = 1
\end{align*}
And since $p^*_i \ge 0$ for all $i$, it immediately follows that $p^*_i \leq 1$ as well.

We now show $N(k^*) = \min_{c\in\Delta_{n-m}} f(p^*, c)$. To this end,
\begin{align*}
f(p^*, c)
    =& \sum_{i\leq n} (c_i(g_i + \ell_i) - \ell_i) p_i \\
%    =& \sum_{i\leq k^*} (c_i(g_i + \ell_i) - \ell_i) \frac{1}{H_{k^*}(g_i+\ell_i)} \\
    =& \sum_{i\leq k^*} \frac{c_i(g_i + \ell_i) - \ell_i}{H_{k^*}(g_i+\ell_i)} \\
    =& \sum_{i\leq k^*} \frac{c_i(g_i + \ell_i)} {H_{k^*}(g_i+\ell_i)}
     - \sum_{i\leq k^*} \frac{(g_i+\ell_i)}{H_{k^*}(g_i+\ell_i)}
     + \sum_{i\leq k^*} \frac{g_i}{H_{k^*}(g_i+\ell_i)} \\
%    =& \sum_{i\leq k^*} \frac{c_i}{H_{k^*}}
%        - \sum_{i\leq k^*}  \frac{\ell_i}{H_{k^*}(g_i+\ell_i)} \\
%    =& \frac{1}{H_{k^*}}\sum_{i\leq k^*} c_i
%        - \sum_{i\leq k^*}  \frac{g_i+\ell_i-g_i}{H_{k^*}(g_i+\ell_i)} \\
    =& \frac{1}{H_{k^*}}\sum_{i\leq k^*} c_i
        -\frac{k^*}{H_{k^*}} 
        + \frac{G_{k^*}}{H_{k^*}}
\end{align*}
Clearly, for $c^*\in\Delta_{n-m}$, this expression is minimized when $c_i = 1$ for $i>k^*$ and $\sum_{i\leq k^*} c_i = k^*-m$. So we have
\begin{align*}
\min_{c\in\Delta_{n-m}} f(p^*, c)
    &= \frac{1}{H_{k^*}}(k^*-m)
        -\frac{k^*}{H_{k^*}} 
        + \frac{G_{k^*}}{H_{k^*}} \\
    &= \frac{G_{k^*} - m}{H_{k^*}} = N(k^*)
\end{align*}
as claimed.
\end{proof}

We now prove our second claim.
\begin{proof}[Proof of Claim~\ref{claim:c}]
We first show that $N(k^*) \ge g_i$ for $i>k^*$.\footnote{In the border case that $k^*=n$, we can add a dummy item with $g_{n+1}=0$ and the claim follows trivially.}
Observe that if $\frac{a}{b} \ge \frac{a+c}{b+d}$, then $\frac{a}{b} \ge \frac{c}{d}$ for non-negative values (and $b>0, d>0$).
Notice
\begin{align*}
\frac{G_{k^*}-m}{H_{k^*}} = N(k^*)\ge  
N(k^*+1) =\frac{G_{k^*}+g_{k^*+1}/(g_{k^*+1}+\ell_{k^*+1})-m}{H_{k^*}+1/(g_{k^*+1}+\ell_{k^*+1})} 
\end{align*}
By our observation,
$$
N(k^*) \ge \frac{g_{k^*+1}/(g_{k^*+1}+\ell_{k^*+1})}{1/(g_{k^*+1}+\ell_{k^*+1})} = g_{k^*+1} \ge g_i \mbox{\ \ for $i>k^*$.}
$$
Similarly, we show $N(k^*) \le g_i$ for $i\leq k^*$, using the observation that if $\frac{a-c}{b-d} \leq \frac{a}{b}$, then $\frac{a}{b} \le \frac{c}{d}$ for non-negative values (and $b-d>0$ and $d>0$).
Notice
\begin{align*}
N(k^*-1) = 
\frac{G_{k^*}-g_{k^*}/(g_{k^*}+\ell_{k^*})-m}{H_{k^*}-1/(g_{k^*}+\ell_{k^*})} 
\leq \frac{G_{k^*}-m}{H_{k^*}}
= N(k^*)
\end{align*}
And again, by our observation,
\begin{equation}
\label{eqn:observation}
N(k^*) \le \frac{g_{k^*}/(g_{k^*}+\ell_{k^*})}{1/(g_{k^*}+\ell_{k^*})} = g_{k^*} \le g_i \mbox{\ \ for $i\le k^*$.}
\end{equation}
Now we're ready to prove the claim.

We first show $c^*\in\Delta_{n-m}$. Since $N(k^*) \le g_i$ for $i\le k^*$, we see
$c^*_i = \frac{N(k^*)+\ell_i}{g_i + \ell_i} \le 1$ for $i\le k^*$. So $c^*_i \in [0, 1]$. Further,
\begin{align*}
\sum_{i\le n} c^*_i
    =& \sum_{i\le k^*} \frac{N(k^*)+\ell_i}{g_i + \ell_i} + \sum_{k^* < i \le n} 1 \\
    =& \sum_{i\le k^*} \frac{N(k^*)-g_i}{g_i + \ell_i} + \sum_{i\le k^*}\frac{g_i+\ell_i}{g_i + \ell_i}  +\sum_{k^* < i \le n} 1 \\
    =& N(k^*) H_{k^*} - G_{k^*} + n \\
    =& G_{k^*} - m - G_{k^*} + n = n-m
\end{align*}
That is, $c^*\in\Delta_{n-m}$.

Finally, we show $N(k^*) = \max_{p\in\Delta_1} f(p, c^*)$. Note that 
$c^*_i(g_i+\ell_i) - \ell_i = N(k^*)$
for $i\le k^*$, while 
$c^*_i(g_i+\ell_i) - \ell_i = g_i$ for $i> k^*$.
We have
\begin{align*}
f(p, c^*) 
    =& \sum_i (c^*_i(g_i + \ell_i) - \ell_i) p_i\\
    =& \sum_{i\leq k^*} N(k^*) p_i
        +\sum_{i> k^*} g_i p_i
\end{align*}
From above, $N(k^*) \ge g_i$ for $i>k^*$. So the expression is maximized for $p\in\Delta_1$ when $p_i = 0$ for $i> k^*$ and $\sum_{i\leq k^*} p_i = 1$. Hence,
\begin{align*}
\max_{p\in\Delta_1} f(p, c^*) = N(k^*)
\end{align*}
as we wanted.
\end{proof} %% End proof of claim.
\end{proof} %% End proof of lemma.

\ignore{
\subsection{Graveyard}

\begin{align*}
N(k^*) &\geq N(k^*+1) \\
\frac{k-M}{H_{k^*}} &\geq \frac{k-M+1}{H_{k^*} + 1/g_{k^*+1}}\\
(k-M)(H_{k^*} + 1/g_{k^*}) & \geq (k-M + 1) H_{k^*} \\
(k-M)/g_{k^*} &\geq H_{k^*} \\
N(k^*) &\geq g_{k^*}
\end{align*}
}  %% end ignore
